# Supplementary material for: Free Space Optical Frequency Comparison Over Rapidly Moving Links
Source: arXiv:2402.08899 ancillary file (2024-06-24)
Supplement: Supplementary file 1 [file supplemental_material.pdf]

# Supplemental Material: Free Space Optical Frequency Comparison Over Rapidly Moving Links

Shawn M. P. McSorley[1], Benjamin P. Dix-Matthews[1], Alex M. Frost[1], Ayden S. McCann[1], Skevos F. E. Karpathakis[1], David R. Gozzard[1], Shane M. Walsh[1], Sascha W. Schediwy[1]

[1]International Centre for Radio Astronomy Research, The University of Western Australia, Crawley, WA 6009, Australia

## S1 Expanded experimental layout

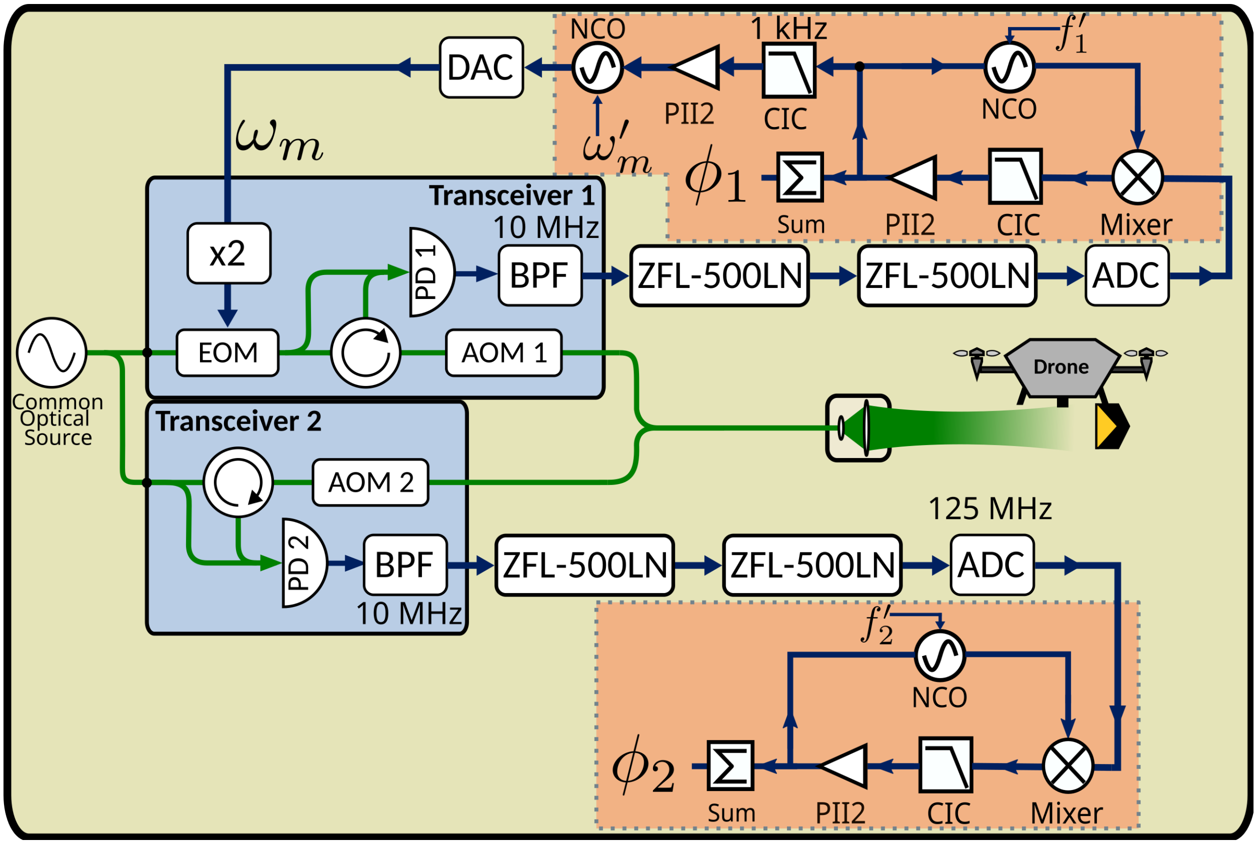


Figure S1: Complete signal chain for the experimental demonstration. Digital control is implemented in the Red Pitaya STEMlab 125-14. EOM, electro-optic modulator; AOM, acousto-optic modulator; PD, photodetector; BPF, bandpass filter; ZFL-500LN, Mini circuits low noise amplifier; ADC, analog-to-digital convert; DAC, digital-to-analog converter; NCO, numerically controlled oscillator; CIC, decimating cascaded integrator comb filter; PII2, proportional integral integral squared; $\omega_m'$, nominal EOM drive frequency; $f_1'$, nominal PD1 heterodyne frequency; $f_2'$, nominal PD2 heterodyne frequency; $f_1$, measured PD1 heterodyne frequency; $\phi_1$, measured PD1 heterodyne phase; $\phi_2$, measured PD2 heterodyne phase. For the experimental demonstration, the AOM drive frequencies are nominally set to $\omega_1 = 48\,\text{MHz}$ and $\omega_2 = -82.5\,\text{MHz}$. The EOM drive frequency is nominally set to $\omega_m' = 22.5\,\text{MHz}$, and doubled to 45 MHz. The nominal heterodyne frequency for PD1 and PD2 are then $f_1' = 10.5\,\text{MHz}$ and $f_2' = 10.5\,\text{MHz}$ respectively. This combination of frequency values was chosen to spectrally separate unwanted optical reflections from the desired signal. As the maximum Doppler shift exceeded 15 MHz, a frequency doubler was used to keep the drive frequency within the Nyquist limit of the Red Pitaya. Not shown is a 10 MHz NCO used to provide an external reference to a signal generator. This signal generator was used to drive the AOMs.

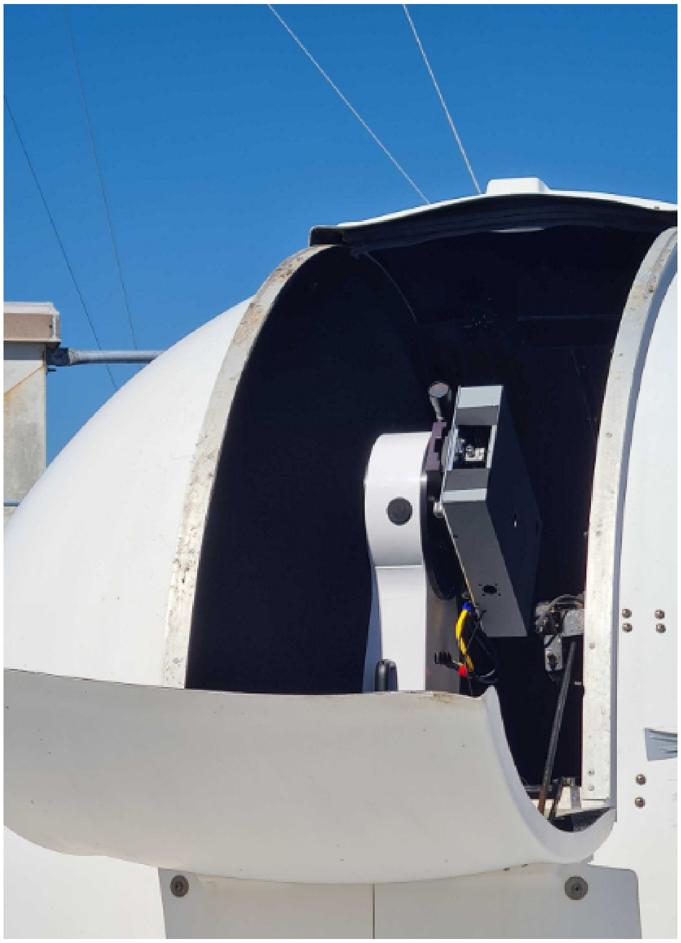

Figure S2: Active terminal located on the roof of the Physics building at the University of Western Australia.

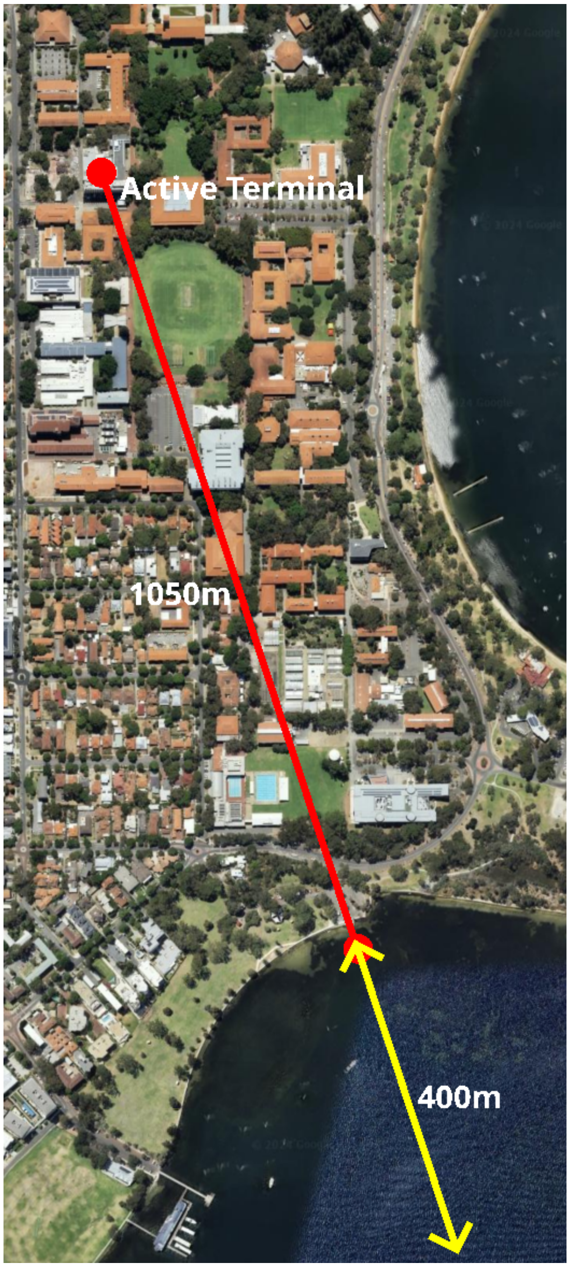


Figure S3: Flight path for the experiment. Labelled are the location of the tracking terminal, the starting position of the drone (red line) and the drone's flight path (yellow). The drone was flown forward and backwards along the yellow path, with a travel of approximately 400 m. The initial distance of the drone, is approximately 1 km away from the terminal. Map generated with Google Earth [1].

## S2 Taylor expansion of ground-to-LEO Doppler shifts

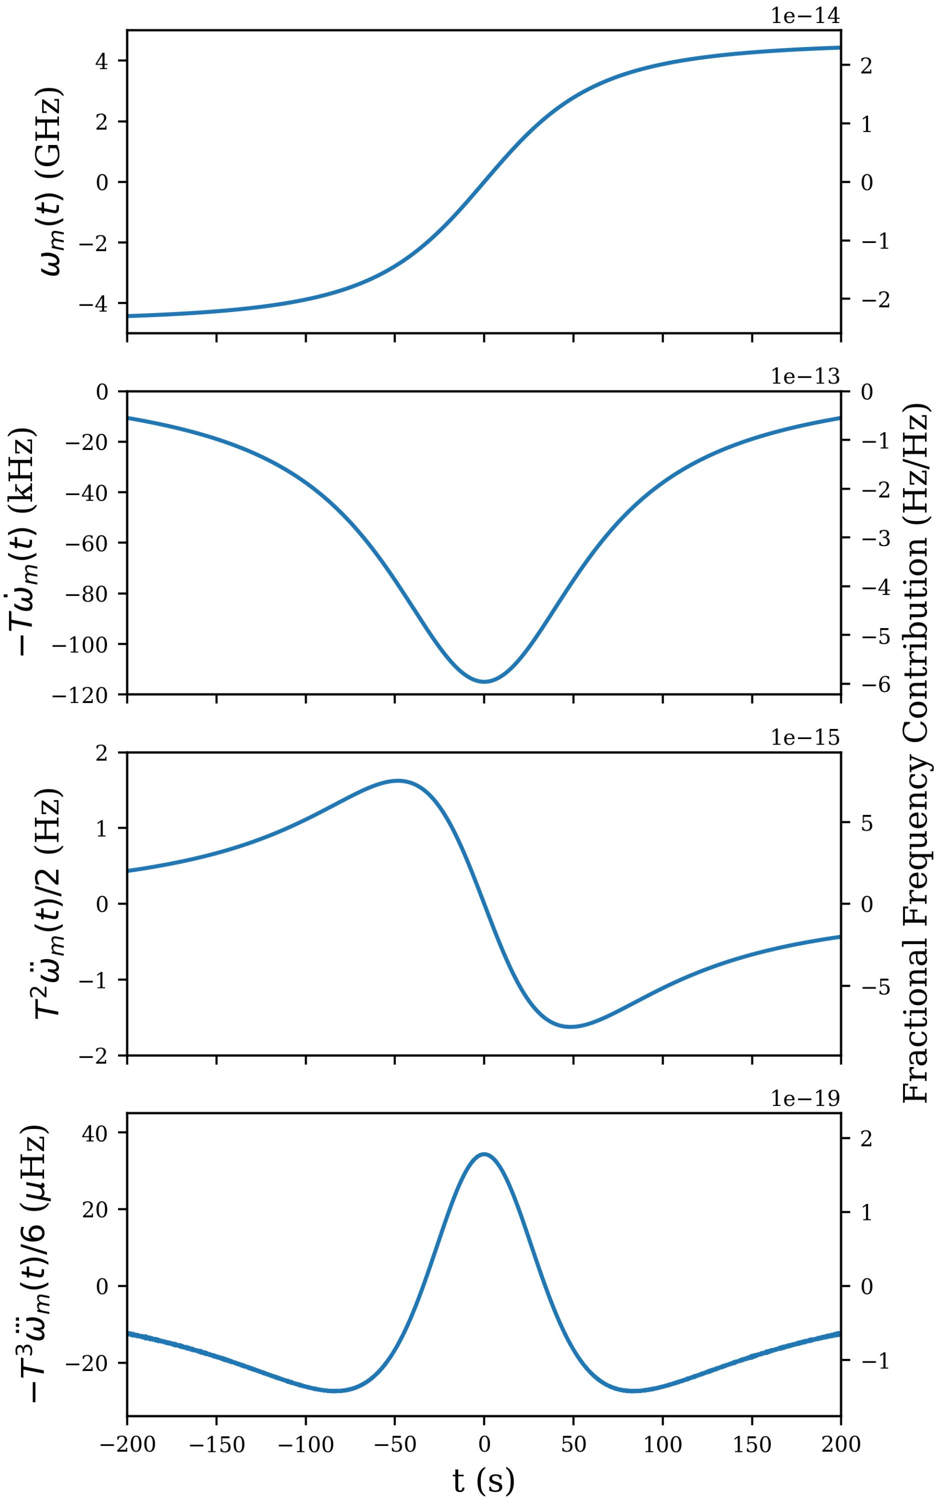


Figure S4: The taylor expansion of the time-delayed EOM drive frequency is $\phi_m(t-T(t)) = \phi_m(t) - T(t)\omega_m(t) + \frac{T^2}{2}\omega_m(t) + \ldots$, where $\omega_m(t) = \frac{d\phi_m(t)}{dt}$. Shown are the expected frequency contributions to $\Delta\phi_L(t)$, determined from Equation 4 in the manuscript, for a ground-to-LEO satellite link, with a velocity of $7600\,\mathrm{m\,s^{-1}}$ and altitude of 500 km. The fractional frequency contribution, for a 1550 nm optical source are also provided on the right axis. For optical frequency comparison on the $1 \times 10^{-18}$ level, this plot indicates that the taylor expansion used for Equation 4, must be at minimum to the third order. The simulated orbital pass start with zenith is at $t = 0$.

# S3 Analysis of sensitivity to initial time-of-flight estimate

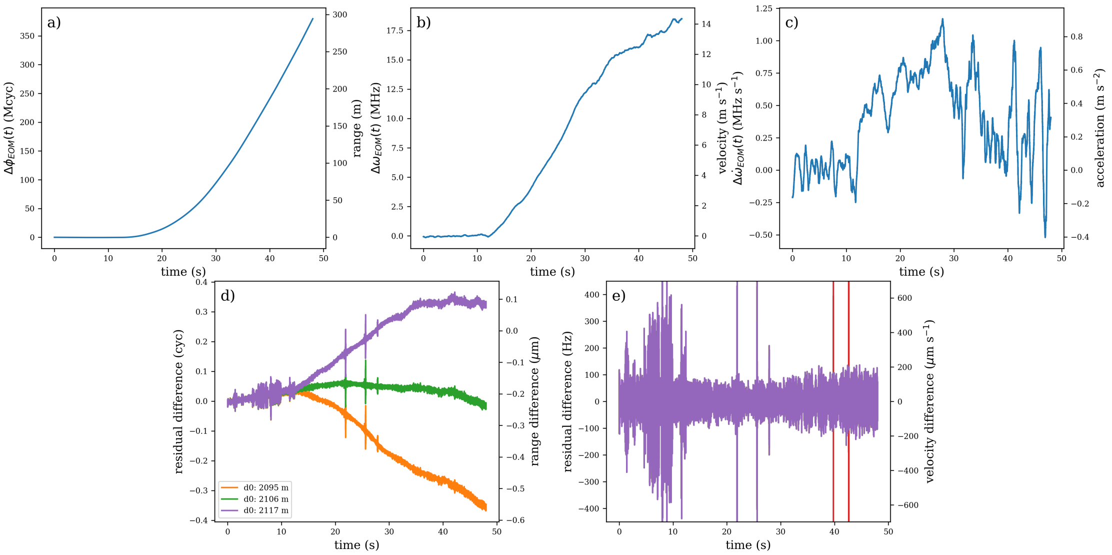


Figure S5: Time series obtained for a drone pass with maximum speed of 15 m s$^{-1}$ and Doppler shift of 20 MHz. Shown on the left-hand y-axes: (a) the accumulated phase of the tracking EOM; (b) the instantaneous frequency of the tracking EOM; (c) the time derivative of the tracking frequency; (d) the residual phase differences with different initial time-of-flight estimates; (e) the instantaneous residual frequency difference for plot (d) and masked cycle slips (red). In plot (e), frequency impulses exceeding 800 Hz, shown in brown, are masked for each time series. In plot (d) and (e), three initial time-of-flight, $T_0$, estimates are provided. The initial $T_0$ is used to calculate the residual correction term $-T(t)\Delta\dot{\phi}_m(t)$ in Equation (4) of the manuscript. Shown on the right-hand y-axes are the associated time-of-flight parameters, with phase corresponding to range, frequency corresponding to velocity, and the time derivative of frequency corresponding to acceleration.

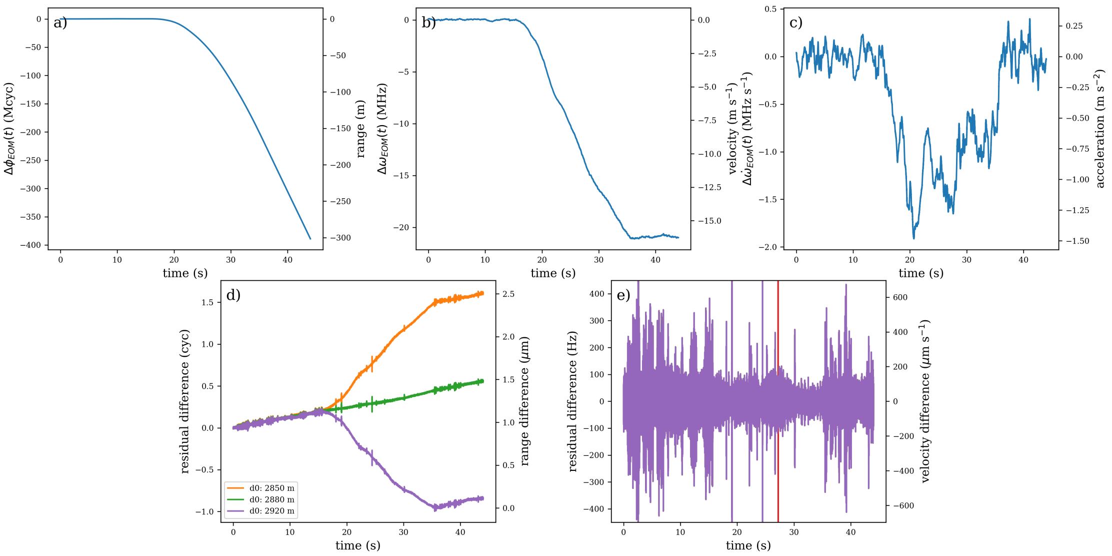


Figure S6: Time series obtained for a drone pass with maximum speed of 17 m s$^{-1}$ and Doppler shift of 21 MHz. Shown on the left-hand y-axes: (a) the accumulated phase of the tracking EOM; (b) the instantaneous frequency of the tracking EOM; (c) the time derivative of the tracking frequency; (d) the residual phase differences with different initial time-of-flight estimates; (e) the instantaneous residual frequency difference for plot (d) and masked cycle slips (red). In plot (e), frequency impulses exceeding 800 Hz, shown in brown, are masked for each time series. In plot (d) and (e), three initial time-of-flight, $T_0$, estimates are provided. The initial $T_0$ is used to calculate the residual correction term $-T(t)\Delta\dot{\phi}_m(t)$ in Equation (4) of the manuscript. Shown on the right-hand y-axes are the associated time-of-flight parameters, with phase corresponding to range, frequency corresponding to velocity, and the time derivative of frequency corresponding to acceleration.

# S4 Analysis of thermal sensitivity

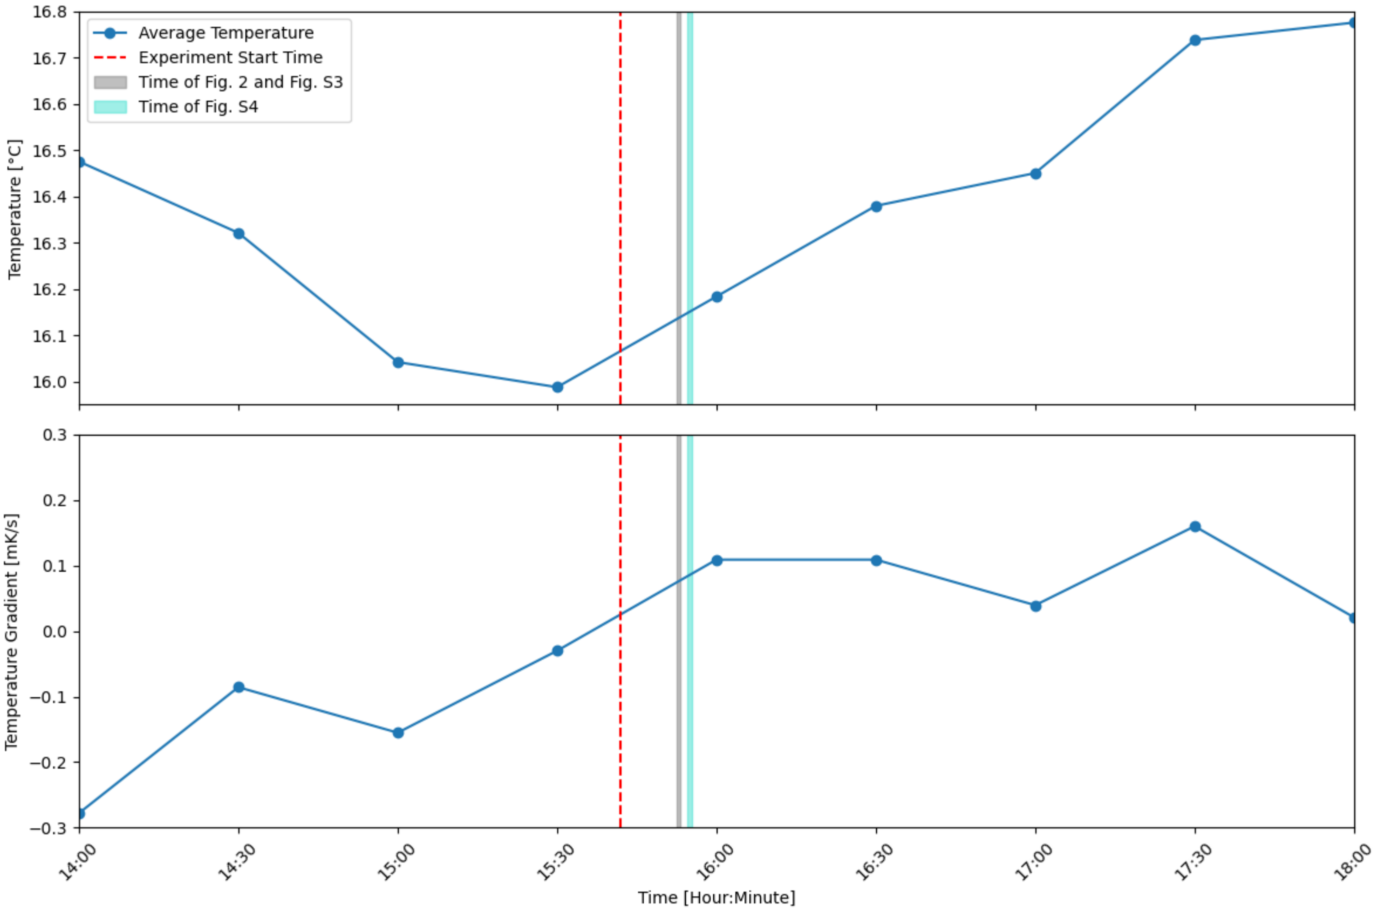


Figure S7: Average temperature and temperature gradient for Perth WA, on the day of 29 September 2023. The dashed red line indicates the start time of the experiment, while the shaded gray box indicates the time of the drone pass shown in Fig. 2 of the Manuscript and Fig. S3, and the shaded blue box indicates the time of the drone pass shown in Fig. S4. The temperature gradient data can be used to determine the thermal sensitivity of the system. At the time of the first drone pass, the temperature gradient was approximately $0.08\,\mathrm{mK\,s^{-1}}$. However, thermal lag of the optical fibers could mean that the temperature gradient could be closer to the maximum value of $-0.3\,\mathrm{mK\,s^{-1}}$ [19]. A change in temperature, $\Delta\bar{T}(t)$, will contribute out-of-loop phase given by $\Delta\phi_L(t) = (n_{T_0}(\alpha+\eta)L_0/\lambda)\Delta\bar{T}(t)$, where $n_{T_0} = 1.4515$ is the refractive index of silica, $\alpha = 10\times10^{-6}\,\mathrm{K^{-1}}$ is the coefficient of thermal expansion for single-mode fiber, $\eta = 7\times10^{-6}\,\mathrm{K^{-1}}$ is the thermo-optic coefficient of silica, $L_0 < 1\,\mathrm{m}$ is the length of out of loop fiber, and $\lambda = 1550\,\mathrm{nm}$ is the wavelength of the optical source. This will provide a frequency drift given by $\Delta\ddot{\phi}_L(t) = (n_{T_0}(\alpha+\eta)L_0/\lambda)\Delta\ddot{\bar{T}}(t)$. From the temperature graident, we can estimate the second derivative of the temperature gradient to be $\Delta\ddot{\bar{T}}(t) \approx 0.1\,\mathrm{\mu K/s^2}$, with a frequency drift of $0.7\,\mathrm{\mu Hz\,s^{-1}}$. This is much less than the observed drift in Fig. 2 of the Manuscript. Rather, the thermal sensitivity of the quartz oscillator used to reference the experiment can be determined from its stability specifications as $125\,\mathrm{MHz}\times 50\ \mathrm{ppm}/125\,\mathrm{K} = 50\,\mathrm{Hz\,K^{-1}}$. This thermal sensitivity would at worst contribute a frequency drift of $50\,\mathrm{Hz\,K^{-1}}\times 0.1\,\mathrm{mK\,s^{-1}} = 5000\,\mathrm{\mu Hz\,s^{-1}}$. Therefore, it is likely that the observed drift in Fig. 2 of the Manuscript is from the quartz oscillator.

# References


[1] Google Earth V 10.55.0.1 (imagery from 2/23/2022–1/16/2024). Nedlands, Western Australia. 31°59'00"S 115°49'05"E, Camera height 2,512m. Airbus. https://earth.google.com [June 21, 2024].
